# Supplementary material for: Reducing information dependency does not cause training data privacy. Adversarially non-robust features do
Source: arXiv:2607.12354 source file (2026-08-07)
Supplement: Supplementary file 1 [file APPENDIX_runtimes.tex]

[moved to APP\_-AT-AT\_masklayer.tex]

% %% Placeholders for Rasmus's runtimes
% \subsection{Deferred discussion of AT-AT practical runtimes} \textbf{AT-AT}'s runtimes are roughly 30\% faster than vanilla AT trained via PGD, because AT requires resistance to strong (high-$\varepsilon$) attacks, whereas AT-AT seeks to learn from imperceptibly subtle (low-$\varepsilon$) features, which require many fewer iterations of PGD. Specifically, a typical research implementation of AT uses a default of $10$ steps of PGD, whereas we used just $3$ to $5$ steps for AT-AT throughout our experiments. These PGD step counts are the practical runtime bottleneck. To be concrete, this translates to runtimes of $3.10$ hours (AT) vs. $2.14$ hours (AT-AT) for CelebA on ResNet-18 architectures (note that all algorithms train for exactly $100$ epochs throughout our experiments). Importantly, like AT, our AT-AT could potentially also benefit from the same well-studied algorithmic and implementation speedups that are widely applied in industry-scale AT implementations \citep[e.g.][]{wong_fast_2020, shafahi_adversarial_2019}. As such, AT-AT can be implemented at scale at significantly lower cost than the AT implementations already in widespread industry use.
% %CelebA R18 runtimes:
% % NoDef: 47 min
% % MID: 48 min
% % BiDO: 57 min
% % RoLSS: 47 min
% % TL-DMI: 38 min
% % AT: 3 hours and 6 min
% % AT-AT: 2 hours and 9 min
