# Supplementary material for: Reducing information dependency does not cause training data privacy. Adversarially non-robust features do
Source: arXiv:2607.12354 source file (2026-08-07)
Supplement: Supplementary file 2 [file old_APPENDIX_AA_accuracy_tables.tex]

% \section{Deferred full results from AutoAttack and adversarial robustness experiments}
% \label{app:AAtables}

% Tables \ref{tab:AA-full-031-formatted}, \ref{tab:AA-full-0025-formatted}, \ref{tab:AA-full-0005-formatted}, \ref{tab:AA-full-1e-05-formatted} present the full results of the AutoAttack adversarial robustness experiments for $\epsilon\in \{0.031, 0.0025, 0.0005, 0.00001\}$, respectively. Specifically, for each of these values of $\epsilon$, the respective table reports robust accuracy of each defense on each dataset and architecture both (1) overall (i.e. worst-case), and for each of standard AutoAttack's four constituent attacks: untargeted Auto-PGD; targeted DLR Auto-PGD \citep{croce_reliable_2020}; FAB \citep{croce_minimally_2020}; and Square \citep{andriushchenko_square_2020}. 


% % Formatted AA Tables:
% \input{dareDEVALII/Tables/AA-FORMATTED-0.031}
% \input{dareDEVALII/Tables/AA-FORMATTED-0.0025}
% \input{dareDEVALII/Tables/AA-FORMATTED-0.0005}
% \input{dareDEVALII/Tables/AA-FORMATTED-1e-05}
